# Supplementary material for: Mechanochemical feedback drives complex inertial dynamics in active solids
Source: arXiv:2505.18272 ancillary file (2025-12-25)
Supplement: Supplementary file 1 [file SI.pdf]

# Supplementary Material:
# Mechanochemical feedback drives complex inertial dynamics in active solids

## I. DERIVATION OF REACTION RATE IN ACTIVE MECHANOCHEMICAL SOLIDS

In this section, we derive Eq. (3) in the main text, where

$$\partial_t \chi = r_+ - r_- = r_{\rm eq} + \zeta\sigma \tag{S1}$$

where $r_{\rm eq} = (k_0/k_BT)(\mu_A - \mu_B) = -2k_0[f'(\chi) + C\epsilon]$ is the equilibrium reaction rate including the passive coupling to strain and $\zeta = k_0(h_A - h_B)/k_BT$ is the non-equilibrium coupling to stress.

To do this, we start from a few equations listed in the main text, including the standard reaction rate equations,

$$\begin{aligned} r_+ &= k_0 \exp(\mu_A/k_BT) \\ r_- &= k_0 \exp(\mu_B/k_BT) \end{aligned} \tag{S2}$$

the passive chemical potentials

$$\mu_B^p = -\mu_A^p = k_BT[f'(\chi) + C\epsilon] \tag{S3}$$

and the active chemical potential

$$\mu_A^a = h_A\sigma, \quad \mu_B^a = h_B\sigma. \tag{S4}$$

Using $\mu_i = \mu_i^p + \mu_i^p$ in Eq. (S2), we have

$$\partial_t \chi = r_+ - r_- = k_0 e^{\mu_A^p/k_BT} e^{h_A\sigma/k_BT} - k_0 e^{\mu_B^p/k_BT} e^{h_B\sigma/k_BT}. \tag{S5}$$

Assuming that the chemical potential is small, $\mu_i \ll k_BT$, we can Taylor expand the exponential factors and have

$$\begin{aligned} \partial_t \chi = r_+ - r_- &\simeq k_0(1 + \mu_A^p/k_BT)(1 + h_A\sigma/k_BT) - k_0(1 + \mu_B^p/k_BT)(1 + h_B\sigma/k_BT) \\ &\simeq (k_0/k_BT)(\mu_A - \mu_B) + (k_0/k_BT)(h_A - h_B)\sigma, \end{aligned} \tag{S6}$$

where we dropped higher order terms in the last line. This is the same as Eq. (3) in the main text.

## II. HOPF BIFURCATION LINE AND THE TIME-PERIOD FOR THE LIMIT CYCLE

We start with the following set of dynamical equations to understand the behavior of the system in different parameter regimes.

$$\begin{aligned} \dot{U} &= V\ , \\ \dot{V} &= -U - \mathsf{Vi}\, V - X, \\ \dot{X} &= \frac{1}{\mathsf{Ch}}\left(-A_u\, U - A_v\, V + X(1 - X^2)\right) \end{aligned} \tag{S7}$$

Note that we set $\tau_{el} = 1$ in our current analysis.

### A. For $A_v > 0$ and $A_u > 0$

The stability matrix is given by

$$M = \begin{pmatrix} 0 & 1 & 0 \\ -1 & -\mathsf{Vi} & -1 \\ -\frac{A_u}{\mathsf{Ch}} & -\frac{A_v}{\mathsf{Ch}} & \frac{1-3X^2}{\mathsf{Ch}} \end{pmatrix} \tag{S8}$$

For the fixed points where $X = \pm\sqrt{1+A_u}$, we get

$$M = \begin{pmatrix} 0 & 1 & 0 \\ -1 & -\mathsf{Vi} & -1 \\ -\frac{A_u}{\mathsf{Ch}} & -\frac{A_v}{\mathsf{Ch}} & \frac{1-3(1+A_u)}{\mathsf{Ch}} \end{pmatrix} \tag{S9}$$

The locus of the point of Hopf bifurcation determines the bifurcation line. We know at the point of Hopf bifurcation one eigenvalue is real and negative while the other two are purely imaginary and complex conjugate of one another. Thus, at the point of Hopf bifurcation, we can write the eigenvalues of $M$ as $\lambda = \lambda_1$ and $\lambda = \pm i\lambda_2$. It implies that the equation for the characteristic polynomial of $M$ should take the following form at the point of Hopf bifurcation

$$(\lambda + \lambda_1)(\lambda^2 + \lambda_2) = 0,$$
$$\lambda_1\lambda_2 + \lambda_2\lambda + \lambda_1\lambda^2 + \lambda^3 = 0. \tag{S10}$$

To obtain the eigenvalues $\lambda$ of $M$, we set $\det|M - I\lambda| = 0$ that yields

$$\frac{2(1+A_u)}{\mathsf{Ch}} + \frac{2\mathsf{Vi} + \mathsf{Ch} + 3\mathsf{Vi}A_u - A_v}{\mathsf{Ch}}\lambda + \left(\mathsf{Vi} + \frac{2+3A_u}{\mathsf{Ch}}\right)\lambda^2 + \lambda^3 = 0. \tag{S11}$$

Comparing Eq.S10 and Eq.S11, we get

$$\lambda_1 = \mathsf{Vi} + \frac{2+3A_u}{\mathsf{Ch}} \tag{S12}$$

$$\lambda_2 = \frac{2\mathsf{Vi} + \mathsf{Ch} + 3\mathsf{Vi}A_u - A_v}{\mathsf{Ch}} \tag{S13}$$

$$\lambda_1\lambda_2 = \frac{2(1+A_u)}{\mathsf{Ch}} \equiv t_1. \tag{S14}$$

The equation for the bifurcation line can be obtained by solving the consistency condition $\lambda_1 \times \lambda_2 - t_1 = 0$.

$$A_v = \mathsf{Vi}\,(2+3A_u) + \frac{\mathsf{Ch}\,(\mathsf{ViCh} + A_u)}{2 + \mathsf{ViCh} + 3A_u} \tag{S15}$$

In the main text, we used $A_u = 50, \mathsf{Ch} = 100.0$ to study the system's dynamical behavior. For this set of parameters, the bifurcation line in the $(A_v - \mathsf{Vi})$ plane is given by (represented by a white dashed line in Fig. 4(a) of the main article)

$$A_v = 152\mathsf{Vi} + 50\left(2 - \frac{51}{38 + 25\mathsf{Vi}}\right), \tag{S16}$$

The time-period $T$ of the limit cycle is determined by the eigenvalue $\lambda_2$ and can be expressed as $T = \frac{2\pi}{\sqrt{\lambda_2}}$. Substituting Eq. (S15) in Eq. (S21) gives the time period

$$T = \frac{\pi}{\sqrt{\frac{1+A_u}{4+2\mathsf{ViCh}+6A_u}}} \tag{S17}$$

### B. For $A_v = 0$ and $A_u < 0$

As $A_v = 0$, the stability matrix is given by

$$M = \begin{pmatrix} 0 & 1 & 0 \\ -1 & -\mathsf{Vi} & -1 \\ -\frac{A_u}{\mathsf{Ch}} & 0 & \frac{1-3X^2}{\mathsf{Ch}} \end{pmatrix} \tag{S18}$$

Since the fixed points do not depend on $A_v$, we get the same fixed points as we had for $A_v > 0$. Note that for $A_u = -1$ three fixed points coalesce to one fixed point $(U, V, X) = (0, 0, 0)$. To get the equation for the bifurcation line for $A_u \leq -1$ we set $X = 0$ in Eq. (S18) and carry out the same analysis as we did for $A_v > 0$ in Sec. II A. Here, representing the eigenvalues at the bifurcation point as $\lambda' = \lambda'_1$ and $\lambda' = \pm i\lambda'_2$, the equation for the characteristic polynomial yielding the eigenvalues $\lambda'$ of $M$ takes the following form

$$\left(1 - \frac{\mathsf{Vi}}{\mathsf{Ch}}\right)\lambda' + \left(\mathsf{Vi} - \frac{1}{\mathsf{Ch}}\right)\lambda'^2 + \lambda'^3 - \frac{1+A_u}{\mathsf{Ch}} = 0 \tag{S19}$$

Again, comparing the form of Eq. (S10) and Eq. (S19) we get

$$\lambda'_1 = \mathsf{Vi} - \frac{1}{\mathsf{Ch}} \tag{S20}$$

$$\lambda'_2 = 1 - \frac{\mathsf{Vi}}{\mathsf{Ch}} \tag{S21}$$

$$\lambda'_1\lambda'_2 = -\frac{1+A_u}{\mathsf{Ch}} \equiv t'_1. \tag{S22}$$

Solving the consistency condition $\lambda'_1 \times \lambda'_2 - t'_1 = 0$, we get the following equation for the bifurcation line in the $(A_u - \mathsf{Vi})$ plane

$$A_u = \mathsf{Vi}\left(\mathsf{Vi} - \frac{1}{\mathsf{Ch}} - \mathsf{Ch}\right) \tag{S23}$$

Note that for $\mathsf{Vi} = \mathsf{Ch}$ and $\mathsf{Vi} = \frac{1}{\mathsf{Ch}}$ we have $A_u = -1$. In particular, for $\mathsf{Ch} = 100.0$ the bifurcation line in the $(A_u - \mathsf{Vi})$ plane is given by (represented by white dashed line in Fig. 3(a) of the main article)

$$A_u = \mathsf{Vi}^2 - \frac{10001\mathsf{Vi}}{100}. \tag{S24}$$

The time-period $T$ of the limit cycle is given by $T = \frac{2\pi}{\sqrt{\lambda'_2}}$ which yields

$$T = \frac{2\pi}{\sqrt{1 - \frac{\mathsf{Vi}}{\mathsf{Ch}}}} \tag{S25}$$

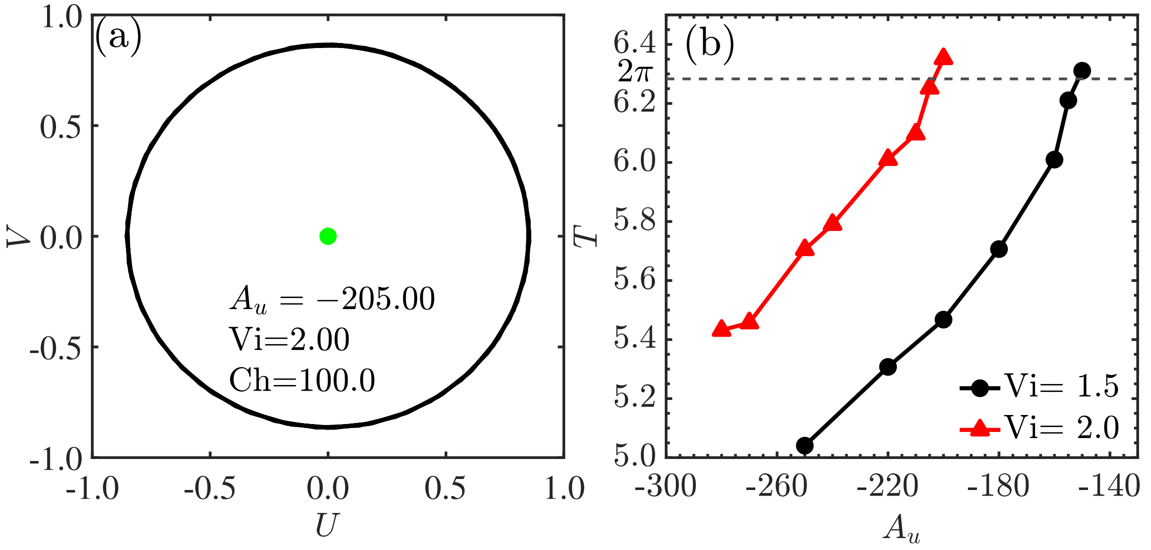


FIG. S-1. (a) Typical trajectory showing a limit cycle (LC) in the overdamped regime ($\mathsf{Vi} > 1, \mathsf{Ch} \gg 1$) for $A_v = 0$ and $A_u < 0$. We set $A_u = -205.0, \mathsf{Vi} = 2.0$, and $\mathsf{Ch} = 100.0$. (b) The dependence of the time period ($T$) of the LC in the overdamped regime on $A_u$ for different values of $\mathsf{Vi}$ with $\mathsf{Ch} = 100$.

Thus, for a fixed $\mathsf{Vi}$, the time-period $T \to 2\pi$ as $\mathsf{Ch} \to \infty$.

Interestingly, this LC behavior persists even in the mechanically overdamped regime ($\mathsf{Vi} > 1, \mathsf{Ch} \gg 1$) with $A_u \ll -1$ as shown in Fig. S-1. We compute the time-period $T$ of such LCs in the overdamped regime and find that the period is also controlled by the same $\tau_{el}$, as long as nonreciprocal feedback dominates the mechanical dissipation rate.

We have two additional fixed points for $A_u > -1$ for $X = \pm\sqrt{1 + A_u}$. To find the bifurcation line for $A_u > -1$ we set $X^2 = 1 + A_u$ in Eq. (S18) and find the following equation for the characteristic polynomial yielding the eigenvalues $\lambda'$

$$\frac{2(A_u+1)}{\mathsf{Ch}} + \lambda' \left(\frac{\mathsf{Vi}(3A_u+2)}{\mathsf{Ch}} + 1\right) + \lambda'^2 \left(\mathsf{Vi} + \frac{3A_u+2}{\mathsf{Ch}}\right) + \lambda'^3 \tag{S26}$$

Representing the eigenvalues at the bifurcation point as $\lambda' = \lambda'_1$ and $\lambda' = \pm i\lambda'_2$, we get

$$\lambda'_1 = \mathsf{Vi} + \frac{3A_u+2}{\mathsf{Ch}} \tag{S27}$$

$$\lambda'_2 = \frac{\mathsf{Vi}(3A_u+2)}{\mathsf{Ch}} + 1 \tag{S28}$$

$$\lambda'_1\lambda'_2 = \frac{2(A_u+1)}{\mathsf{Ch}} \equiv t_2. \tag{S29}$$

The equation for the bifurcation line can be obtained by solving the consistency condition $\lambda'_1 \times \lambda'_2 - t_2 = 0$ and we obtain the following permissible solution for $-1 \leq A_u \leq 0$

$$A_u = -\frac{\mathsf{Ch} + 12\mathsf{Vi} + 3\mathsf{Vi}^2\mathsf{Ch} - \sqrt{\mathsf{Ch}}\sqrt{3\mathsf{Vi}\left(3\mathsf{Vi}^3\mathsf{Ch} - 10\mathsf{Vi}\mathsf{Ch} + 8\right) + \mathsf{Ch}}}{18\mathsf{Vi}} \tag{S30}$$

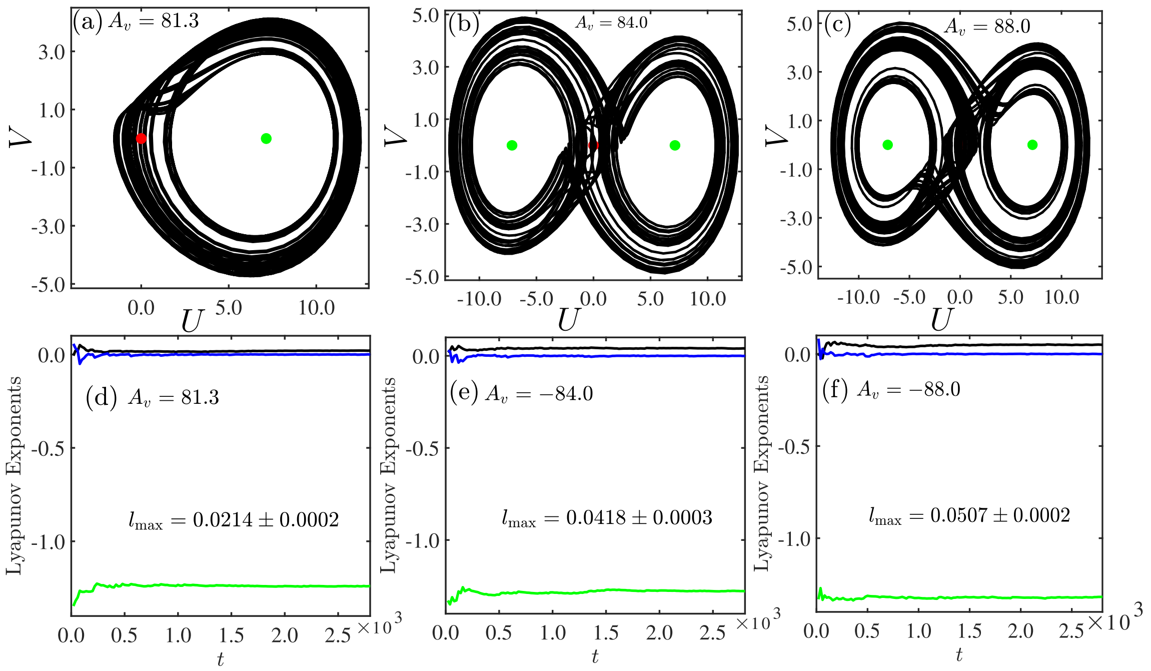


FIG. S-2. Typical chaotic trajectories in the $(U, V)$ plane for (a) $A_v = 81.3$, (b) $A_v = 84.0$, and (c) $A_v = 88.0$. In all cases, we set $A_u = 50, \mathsf{Vi} = 0.16$, and $\mathsf{Ch} = 100$. (d-f) The time-dependence of the three Lyapunov exponents for the trajectories shown in (a-c), respectively. A positive value for the largest Lypunov exponent $l_{\max}$ in each case confirms the chaotic nature of the trajectory.

Thus, for a given $\mathsf{Ch}$ Eq. (S30) gives the bifurcation line for $-1 \leq A_u \leq 0$ while Eq. (S23) represents the bifurcation line for $A_u \leq -1$ with $A_v = 0$. Note that for $\mathsf{Vi} = \frac{1}{\mathsf{Ch}}$ Eq. (S23) and Eq. (S30) yields $A_u = -1$.

For $\mathsf{Ch} = 100$, we get the bifurcation line shown in the main text

$$A_u = -\frac{150\mathsf{Vi}^2 + 6\mathsf{Vi} + 50 - 10\sqrt{3\mathsf{Vi}\left(75\mathsf{Vi}^3 - 250\mathsf{Vi} + 2\right) + 25}}{9\mathsf{Vi}}. \tag{S31}$$

At $\mathsf{Vi} = 0.01(= \frac{1}{\mathsf{Ch}})$ we get $A_u = -1$ from Eq. (S31) and Eq. (S23) implying that the bifurcation line is continuous in the $(A_u - \mathsf{Vi})$ plane for $A_u \leq 0$.

## III. LYAPUNOV EXPONENTS

To analyze the nature of the trajectory in the chaotic regime, we compute the Lyapunov exponents, a quantity that characterizes the rate of separation of infinitesimally close trajectories [s1]. As the phase space is three-dimensional $(U, V, X)$ we have three Lyapunov exponents. A positive value for the maximal Lyapunov exponent is usually taken as an indication that the system is chaotic for the given parameter regime. We study the time-dependence of the three Lyapunov exponents for different parameter values chosen from the chaotic regime in phase diagram Fig. 4(a). The typical

chaotic trajectories in the $(U, V)$ plane are shown in Fig. S-2 for (a) $A_v = 81.3$, (b) $A_v = 84.0$, and (c) $A_v = 88.0$. In all cases, we set $A_u = 50.0, \mathsf{Vi} = 0.16$, and $\mathsf{Ch} = 100$ (see Fig. 4(a) for the identification of the chaotic regime). For each trajectory we compute the time dependence of three Lyapunov exponents using MATCONT [s2] as shown in Fig. S-2(d-f). All Lyapunov exponents saturate at large $t$, and we compute the average value of the Lypunov exponents by taking the average of the instantaneous values of the Lyapunov exponents in the final 1000 time steps. We find that the maximal Lyapunov exponent $l_{\max} > 0$ for all the trajectories chosen in the aforementioned parameter regimes implies that the system exhibits chaotic dynamics in these parameter regimes.


[s1] Steven H Strogatz, *Nonlinear dynamics and chaos: with applications to physics, biology, chemistry, and engineering* (Chapman and Hall/CRC, 2024).

[s2] A. Dhooge, W. Govaerts, and Yu. A. Kuznetsov, "Matcont: A matlab package for numerical bifurcation analysis of odes," ACM Trans. Math. Softw. **29**, 141–164 (2003).
